# Supplementary material for: Building Extensible Program Logics through Effect Handlers (Extended Version)
Source: arXiv:2607.12642 source file (2026-11-30)
Supplement: Supplementary file 1 [file transformer.tex]

\section{The Protocol Aligning Algorithm}\label{sec:app:proofmode}

\subsection{Protocol Transformers}\label{app:transformer}

A protocol transformer $\mathcal{T}$ is a function from protocols to protocols such that
\begin{mathpar}
\inferrule[T-Mono]
{}
{\Psi_1\sqsubseteq\Psi_2\vdash\mathcal{T}(\Psi_1)\sqsubseteq\mathcal{T}(\Psi_2)}\and
\inferrule[T-Sum]
{}{\mathcal{T}(\Psi_1\oplus\Psi_2)\equiv\mathcal{T}(\Psi_1)\oplus\mathcal{T}(\Psi_2)}
\end{mathpar}

Expanding transformer: $\mathcal{T}(\Psi)\sqsubseteq\Psi$

Restricting transformer: $\Psi\sqsubseteq\mathcal{T}(\Psi)$
